# Supplementary material for: Spiking Neural Networks modelled as Timed Automata with parameter learning
Source: arXiv:1808.01893 source file (2018-08-01)
Supplement: Supplementary file 1 [file appendix.tex]

% !TEX root = mainjournal.tex

	\subsection{Non-deterministic input sequences.}	 \label{subsec:nondet-input}
		
		\begin{figure}[t]
			\centering
			\includegraphics[scale=0.5]{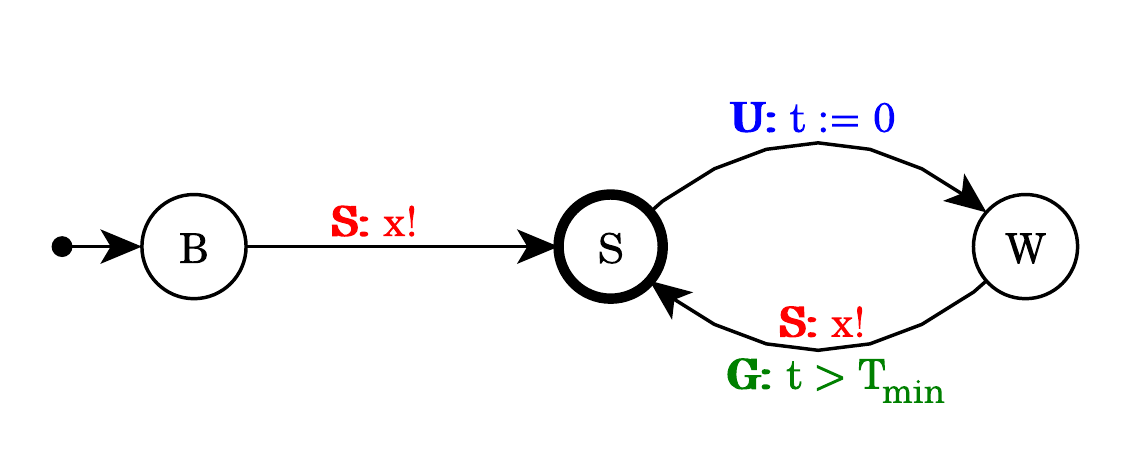}
			\caption{Non-deterministic input sequence automaton}
			\label{fig.ta.nondeterministic_generator}
		\end{figure}%

		Non-deterministic input sequences are valid input sequences where the occurrence times of spikes is random but the minimum inter-spike quiescence duration is $T_{min}$. 	
\input{newsimulation.tex}
